# Supplementary material for: A Local-to-Global Approach to Multi-modal Movie Scene Segmentation
Source: arXiv:2004.02678 source file (2020-04-28)
Supplement: Supplementary file 1 [file supp.tex]

% !TEX root = ../main.tex

\clearpage

\section{Details of Global Optimal Grouping}

\subsection{Scene cut score}
The scene cut score achieved by one scene is defined as follows,
\begin{align*}
g(l_{k}, r_{k}) = 
\sum_{\tilde{s}_{i_k} \in \mathcal{C}_k} 
f(\tilde{s}_{i_k},\mathcal{P}_{k}),
\end{align*}
where
$$
f(\tilde{s}_{i_k},\mathcal{P}_{k}) = \alpha(|\mathcal{P}_{k}|)(F_s(\tilde{s}_{i_k},\mathcal{P}_{k}) + F_t(\tilde{s}_{i_k},\mathcal{P}_{k})).
$$
$$
F_s(\tilde{s}_{i_k},\mathcal{P}_{k})= \frac{1}{|\mathcal{P}_{k}|} \sum_{j_k \in \mathcal{P}_{k}} \cos (\tilde{s}_{i_k},\tilde{s}_{j_k}),
$$
$$
F_t(\tilde{s}_{i_k},\mathcal{P}_{k})= \sigma(\max_{j_k \in \mathcal{P}_{k}} \cos (\tilde{s}_{i_k},\tilde{s}_{j_k})),
$$
Notice that $\mathcal{P}_{k}$ is the preceding part of that of shots $\{s_{l_{k}},\cdots,s_{i_{k}} \}$ before $s_{i_{k}}$, and $\alpha$ is a decay factor to prevent the scene from growing too large. $f(\tilde{s_{i_k}},\mathcal{P}_{k})$ formulate the relationship between a shot ($\tilde{s_{i_k}}$) and a set of shots ($\mathcal{P}_{k}$), we use two term to capture a global relationship and a local relationship, $F_s(\tilde{s_{i_k}},\mathcal{P}_{k})$ is similarity score between the shot $s_{i_k}$ and $\mathcal{P}_{k}$,
and $F_t(\tilde{s_{i_k}},\mathcal{P}_{k})$ is an indicate function that whether there is a very high similarity between the shot $s_{i_k}$ and any shot from $\mathcal{P}_{k}$.\footnote{This is to formulate shots thread in a scene.} $\sigma(\cdot)$ is a sigmoid function.

\subsection{Details of Gradient computation in DP step}
For notation simplicity, we denote the derivatives of cosine similarity $d(i,{i-j}|W_i)$ and $d(i,{i-j}|b_i)$ as follows,
\begin{align*}
&d(i,{i-j}|W_i) \\
& =  \frac{\partial \cos(W_{i}S_{i}+b_i,W_{i-j}S_{i-j}+b_{i-j}) } {\partial W_i} \\
&= ( \frac{W_iS_i+b_i}{|W_{i}S_{i}+b_i||W_{i-j}S_{i-j}+b_{i-j}|}  \\
&- \cos(W_{i}S_{i}+b_i,W_{i-j}S_{i-j}+b_{i-j})\frac{W_iS_i+b_i}{|W_{i}S_{i}+b_i|^2} ) S_i,
\end{align*}

\noindent We update model parameters using the following gradients,
\begin{align*}
&\frac{\partial F } {\partial W_i} 
= \frac{1}{|\mathcal{C}_{k}|} \sum_{j\in \mathcal{C}_{k}} d(i,{i-j}|W_i) \\
&+ \sum_{j\in ((i+1)_k,r_k)} \sum_{i \in \mathcal{M}_{i,j}}
\sigma(  d(i,{i-j}|W_i)) 
(1 - \sigma(  d(i,{i-j}|W_i))),
\end{align*}

where $\mathcal{M}_{i,j} =$ \\
$\{i | i =\arg max \cos(W_{j}S_{j},W_{j-g}S_{j-g}),{g\in (l_k,(j-1)_k)}\} $.

\noindent\textbf{Iterative supers shots mergence.}
Recall the initial scene cut set from local segmentation is $\mC^0 =\{\cC_k^0\} = \cV$.
In the first loop $(p < K_{set})$, we merge the super shots iterative, \ie~$\mC^p \rightarrow \mC^{p+1}$
according to the optimal scene cut result achieved from the dynamic programming.

\noindent\textbf{Super shots representation refinement.}
The representation of a super shot comes from the weighted sum of the shots consist of it, which is defined as $\cC_k^p = W_k^p S_k^p$,
and $S_k^p$ is the shots that constitute of the super shot $\cC_k^p$
\footnote{Recall that in a video, shots constitute super shots, and super shots constitute scenes. }
%	In mathematics notation, \\$\mathcal{V} 
%	= \{s_k\} = \{\{s_1,\cdots,s_{n_1}\} ,\cdots,\{s_{n_{m-1}+1},\cdots,s_{n_m}\} \} \\
%	= \{\cC_k^p\} = \{\{\tilde{s}_1,\cdots,\tilde{s}_{N_1}\}  ,\cdots,\{\tilde{s}_{N_{k-1}+1},\cdots,\tilde{s}_{N_k}\}\}  \\
%	=\{\mathcal{C}^\star_k\} =\mC^\star $.}
, and $W_k^p$ are parameters.
In the second loop $(q < K_{para})$, with the maximum value $F(W)$ achieved in DP, we update $W$ with gradient decent. Through this process, we update the representation of super shots $\cC_k^p = W_k^p S_k^q$.\footnote{Note that the gradient calculation is not trivial since different scene consists of different super shots.
	The detailed derivation of gradients is in the supplements.}

\begin{algorithm}[t]
	\caption{Super shots optimal grouping algorithm}
	\textbf{Input}: coarse scene cut set $\mC^0$ from local segmentation\\
	\textbf{Output}: optimal scene cut set $\mC^*$ \\
	\textbf{Initialization}: current scene cut set $\mC = \mC^0$ \\
	
	\begin{algorithmic}[1]
		\vspace{-10pt}
		\WHILE{$p<K_{set}$}
		\WHILE{$q<K_{para}$}
		\STATE Obtain super shots representation vector $\cC_k^p$ based on parameters $ W_k^p$ and shots $S_k^p$.
		\STATE Get maximum scene cut score $F$ with DP.
		\STATE Update parameters $ W_k^p$ with refinement.
		\ENDWHILE
		\STATE Update current scene segments set $\mC = \mC^{p+1}$ according to $F$.
		\STATE Merge super shots $\cC_k^p$ and $\cC_{k+1}^p$ if $\cC_k^p,\cC_{k+1}^p \in \mathcal{C}_k^{p+1}$.
		\ENDWHILE
	\end{algorithmic}
	\label{alg:dp_supp}
\end{algorithm}
\subsection{Visualization}
We visualize the correlation matrix of super shots in different iteration step in global optimal grouping in one movie as shown in Figure~\ref{fig:global} (iteration $0$,$3$,$5$).
An ideal scene co-relationship map of scenes has a block-wise diagonal part, which means that different scenes share low correlation and the scene segmentation is successful, as shown in the Figure~\ref{fig:model}. In this grouping result, super shots reduce from $600$ (in iteration $0$) to $139$ (in iteration $5$). The diagonal block effect becomes more obvious. 
\begin{figure}[!t]
	\begin{center}
		\includegraphics[width=\linewidth]{imgs/qual_global.pdf}
	\end{center}
	\vspace{-10pt}
	\caption{\small
		Global optimal grouping correlation matrix visualization.
	}
	\label{fig:global}
	\vspace{-10pt}
\end{figure}

\section{Appendix: MovieScenes Statistics}
\begin{figure}[t!]
	\centering 
	\includegraphics[width=0.9\linewidth]{imgs/movie_stats.png}
	\caption{Four selected characteristics of \emph{MovieScenes}. \textit{Left top:} movie length distribution. \textit{Left bottom:} movie genera distribution.  \textit{Right top} and \textit{Right bottom} tells about the general statistical information of scene summarized from the dataset.}
	\label{fig:pi}
	\vspace{-10pt}
\end{figure}

Table~\ref{tab:datastat} shows some basic statistics about our dataset.
Our dataset consists a total of $272,301$ binary decisions from $150$ movies. 
\begin{table}[!t]
	\caption{
		Statistics of the \emph{MovieScenes} annotation set. }
	\vspace{-10pt}
	\begin{center}
		\resizebox{\columnwidth}{!}{
			\begin{tabular}{lrrrr}
				\toprule
				& Train 		&  Val 		& Test 	& Total\\ \midrule
				Number of Movies  		&  100  		&  20  		& 30    &150	\\
				Number of  Scenes		&  14,389  		&  2,338  	& 4,701 & 21,428\\
				Number of  Shots  		&  188,892  	&  23,549  	& 58,009 &270,450 \\ \midrule
				Avg. Dur. of Movie (h) & 2.01    &  1.74    	& 2.02  & 1.98\\
				Avg. Dur. of Scene (s) & 50.00   &  53.33      & 46.08 &49.50 \\
				Avg. Dur. of Shot (s)  & 3.84    &  5.31    	& 3.78  &3.95\\
				\bottomrule
			\end{tabular}
		}
	\end{center}
	\label{tab:datastat}
	\vspace{-10pt}
\end{table}

\subsection{Dataset Consistency}
We divide all annotations into three categories:
(1) \emph{high consistency cases}, \ie~those that received same results from three annotators in the first round or those that received same results from four of the five annotators after the second round. 
(2) \emph{low consistency cases}, \ie~those that received same results
from three of the five annotators after the second round. They are hard cases for human since annotators achieve low consistency;
(3) \emph{unsure cases}, \ie~those are bad cases for human since annotators cannot achieve consistency. We discard this category in the following experiments.
Table~\ref{tab:dataanno} shows the consistency statistics.

\subsection{Annotation Interface}
The annotation interface is shown in Figure~\ref{fig:inter}. Annotators click \emph{MOVIES LIST} to chose a clip to annotate. \emph{MANUAL} shows instructions.
\emph{LANGUAGE SWITCH} switches interface language.

If the central shots pair is a scene transition, annotators press \emph{X} to annotate \emph{Transit}.
If the central shots pair is not a scene transition, annotators press \emph{Z} to annotate \emph{Continue}.
If annotators are unsure about their decision, they press \emph{C} to annotate \emph{Skip}.

The center of the interface are the videos of a shots pair. And the left and right side are two still images. If the annotation is continue, a blue arrow will show between two shots. If the annotation is transit, a red vertical bar will show between two shots. At the top of each shot, there is a indicator that shows the number.
At the bottom, there shows the progress of annotations.

\begin{figure*}[!t]
	\vspace{-0pt}
	\begin{center}
		\includegraphics[scale=0.2]{imgs/inter.png}
	\end{center}
	\vspace{-5pt}
	\caption{\small
		Annotation interface.
	}
	\label{fig:inter}
	\vspace{-0pt}
\end{figure*}

\section{More Qualitative Results}
\begin{figure}[!t]
	\vspace{-10pt}
	\begin{center}
		\includegraphics[scale=0.3]{imgs/res1.png}
	\end{center}
	\vspace{-8pt}
	\caption{\small
		Non-transition cases. Each row represents four consecutive shots from one scene. These scenes from top to bottom are underwater diving, driving fighters, driving helicopters, escorting prisoners, driving cars and dressing. Our model is able to find internal details correlation and give right predictions.
	}
	\label{fig:res1}
	\vspace{-2pt}
\end{figure}

\begin{figure}[!t]
	\begin{center}
		\includegraphics[scale=0.3]{imgs/res2.png}
	\end{center}
	\vspace{-10pt}
	\caption{\small
		Transition cases. Each row represents four consecutive shots from two adjacent scenes. The scene boundary is in the middle of the second and the third shot. Our model is able to recognize salient semantics change and give right predictions.
	}
	\label{fig:res2}
	\vspace{-0pt}
\end{figure}
More qualitative results are shown in Figure~\ref{fig:res1} and~\ref{fig:res2}. Figure~\ref{fig:res1} and~\ref{fig:res2} show non-transition and transition cases respectively, in both of which our model make right predictions.

Although, in Figure~\ref{fig:res1}, four consecutive shots from one scene seemingly have different semantic information, our model can still predict non-transition through some implicit cues, such as role's appearance from different views and relationship between the parts and the whole of an obejct.

Scene transition indicates salient semantics change, thus usually contains sharp visual features change including characters, props, places and light conditions. These changes are relatively easier to recognize. Figure~\ref{fig:res2} shows some transition cases and our successful predictions.

\section{Details of the Extension}
\subsection{Improving Character Recognition}

Character recognition in a movie is a challenging task since a movie contains lots of shots where characters do not show up their full faces, as shown in Figure~\ref{fig:reid}.

With the help of scene, we are able to establish two strong priors to handle these ambiguous cases.
It is known that the characters appeared within one scene must be the same. The character without full faces is likely to be the one shown up with faces in the rest part of the same scene.
Thus we take advantages of \emph{character-scene relationship} to infer those characters without faces.
Additionally, along with the whole movie, \emph{character-character relationship} (\eg~human interaction graph) can be got from Scenes and we are able to know which group of characters is more likely to appear in the same scene. Therefore, in the case that there are two people appearing in one shot with one people showing face and the other one only showing the back, we can leverage the character-character relationship to make prediction for those characters without clear faces.

We conduct experiments on our test set using character label from~\cite{huang2018unifying} and pick out the shots where no faces are detected. 
For each movie, 10 casts are annotated and have annotation in each shot. These 10 casts come from the top of the corresponding movie IMDB profile.
3,000 shots are picked out from 30 movies. These shots are hard cases for traditional methods of character recognition, since there are no clear faces of these characters shown in the shots. 

\begin{figure}[!t]
	\begin{center}
		\includegraphics[scale=0.2]{imgs/reid.pdf}
	\end{center}
	\vspace{-5pt}
	\caption{\small
		Character Recognition. 
		The first row uses the character-scene relationship to recognize the character in red bounding box from the one in green bounding box.
		The second row uses the character-character relationship to recognize the character in red bounding box using the relationship between the one in green bounding box and the one in blue bounding box.
	}
	\label{fig:reid}
	\vspace{-0pt}
	
\end{figure}
\begin{table}[!t]
	\caption{
		Accuracy of character recognition on hard cases. Rand: Random guess; Char: Character-character relationship; Scen: Character-scene relationship; Both: use both character-scene relationship and character-character relationship.}	\begin{center}
		\begin{tabular}{cccccc}
			\toprule
			Method& Rand & \begin{tabular}[c]{@{}c@{}}Char\\ (Shot)\end{tabular} & Scen& Char& Both \\ \midrule
			Accuracy  & 0.09 & 0.20        & 0.29 &0.28 & 0.33   \\ \bottomrule
		\end{tabular}
		\vspace{-5pt}
	\end{center}
	\vspace{-9pt}
	\label{tab:reid}
\end{table}

We use character-scene relationship and character-character relationship as priors to infer character identity, as shown in Table~\ref{tab:reid}. We build character-character relationships based on shots as comparison. And it is unable to build character-scene relationship based on shots.

Since we are only concerned about the 10 casts. So random guess is at 0.09 accuracy on character recognition, while our best method, which use the above two priors, achieve 0.33 accuracy. It is much better than random guess and shot-based character interaction.
It is shown that Scenes help build up a better character-character relationship and combining it with character-scene relationship help to improve performance on the hard cases of character recognition.

\subsection{Generating Human Interaction Graph}
\begin{figure*}[!t]
	\begin{center}
		\includegraphics[width=\linewidth]{imgs/humanint.png}
	\end{center}
	\vspace{-12pt}
	\caption{\small
		Human Interaction Graph.
		The first line is \textit{American Hustle} scene segmentation coming from scene detection, 
		where dark blue and light blue intertwine with each other to represent different Scenes.
		The second to fourth line corresponds to \textit{C.B. Christian Bale; B.C. Bradley Cooper; A.A. Amy Adams} Scenes occurrence time lines in this movie respectively, where the dark green means occurring while light green does not.
		The graph below represents their interaction over the story line. The dark red represents a closer relationship while the light red represents a far-away relationship and two demo pictures are shown for closer relationships.
	}
	\label{fig:humanint}
	\vspace{-8pt}
\end{figure*}
After recognizing characters in shots~\cite{huang2018unifying}, we can group these characters into Scenes according to 
shots-Scenes relationship coming from segmented Scenes. 
Figure~\ref{fig:humanint} visualizes each character occurrence Scenes.
We derive a novel human interaction graph from all characters occurrence, to visualize the evolution of characters' relationships over time. It clearly shows that the characters' interaction develop over time. Furthermore, based on the segmented Scenes, we can count the total character interaction time, \eg~C.B and A.A are with each other fifty minutes in the two hour \textit{American Hustle}.

Shot-based character occurrence counting is much less accurate than the scene-based character occurrence counting, since not all the consecutive shots contain the full face of a character though he/she is inside the scene.

\subsection{Cross Movie Scene Retrieval}

It is still an open question to represent a long video such as the scene. 
A collection of well segmented Scenes can serve as good samples for studying how to organize high-level semantic video reprtneesentation as well
as facilitate the development of methodologies for a number of salient tasks related to semantics understandings, \ie~scene retrieval, language query retrieval and
movie summarization.

Consider the Cross Movie Scene Retrieval, where we are given a specific scene and asked to retrieve similar ones in other movies. For example, given a scene of person chatting in a room, we would like to retrieve all the similar Scenes from all the other movies. The task is of great practical interest and has a variety of real-world applications, \eg~personalized
marketing and intelligent searching. It demands a deep analysis of videos that goes beyond recognizing the visual appearance or simple
action pattern. Compared to a single shot, the segmented scene allows us to extract rich correlated features (\eg~characters, specific objects,
and places) in a self-contained semantic segment. 

As a baseline for cross movie scene retrieval, we extract features from visual cues and characters interaction and compute similarity for every Scenes pair. We take the top similar Scenes as result.
Some example results of the cross movie scene is shown in Figure~\ref{fig:retrieval}. Two characters appear alternately in a conversation scene and there is a long shot which contains these two characters. Lots of character appear in a party scene and there are many extra actors. The neon lights provide a dark and flicking environment.
\begin{figure*}[!t]
	\vspace{-9pt}
	\begin{center}
		\includegraphics[width=\linewidth]{imgs/retrieval.png}
	\end{center}
	\vspace{-15pt}
	\caption{\small
		Cross movie scene retrieval. We choose a conversation scene and a party scene  from \textit{Ted (2012)} as query, then
		retrieve similar Scenes from other movies. 
	}
	\label{fig:retrieval}
	\vspace{-3pt}
\end{figure*}
